# Supplementary material for: Domain Adaptation Using Pseudo Labels
Source: arXiv:2402.06809 source file (2024-03-12)
Supplement: Supplementary file 1 [file X_suppl.tex]

\clearpage
\setcounter{page}{1}
\maketitlesupplementary

\section{Rationale}
\label{sec:rationale}
Having the supplementary compiled together with the main paper means that:
\begin{itemize}
\item The supplementary can back-reference sections of the main paper, for example, we can refer to \cref{sec:intro};
\item The main paper can forward reference sub-sections within the supplementary explicitly (e.g. referring to a particular experiment); 
\item When submitted to arXiv, the supplementary will already included at the end of the paper.
\end{itemize}
To split the supplementary pages from the main paper, you can use \href{https://support.apple.com/en-ca/guide/preview/prvw11793/mac#:~:text=Delete%20a%20page%20from%20a,or%20choose%20Edit%20%3E%20Delete).}{Preview (on macOS)}, \href{https://www.adobe.com/acrobat/how-to/delete-pages-from-pdf.html#:~:text=Choose%20%E2%80%9CTools%E2%80%9D%20%3E%20%E2%80%9COrganize,or%20pages%20from%20the%20file.}{Adobe Acrobat} (on all OSs), as well as \href{https://superuser.com/questions/517986/is-it-possible-to-delete-some-pages-of-a-pdf-document}{command line tools}.

\begin{figure*}[t]
    \begin{center}
      \includegraphics[width = \textwidth]{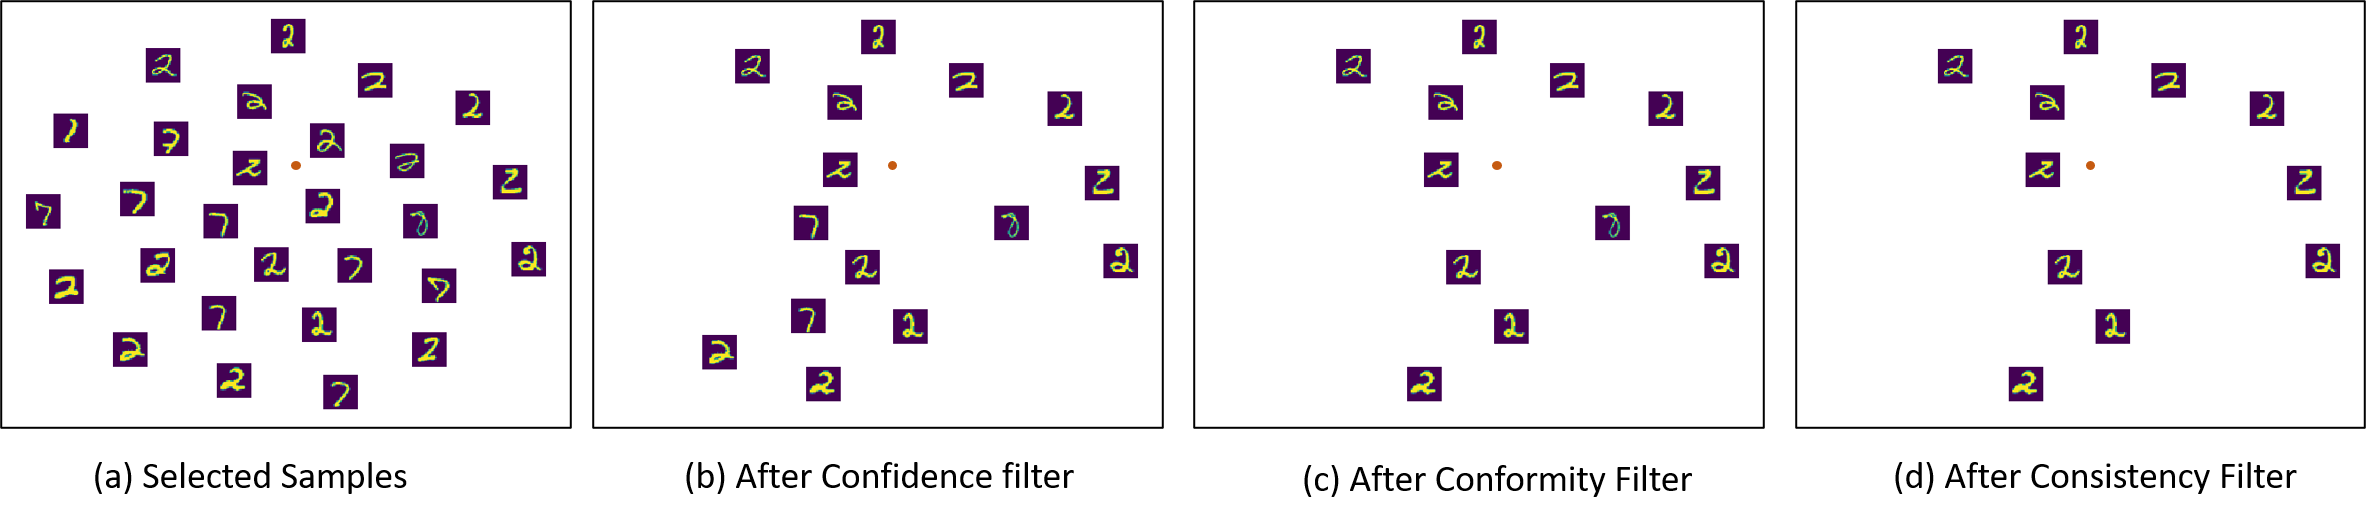}
    \end{center}
\caption{Illustration of the 3-level pseudo label filtering technique for target data using t-SNE plots. These are samples from one mini-batch of data, (a) shows a set of 22 samples with the pseudo label `2' - notice the false positives. (b) After \emph{Confidence} filter (c) After \emph{Conformity} filter (d) After \emph{Consistency} filter}
\label{Fig:filters}
\end{figure*}

\begin{algorithm}
\SetAlgoLined
\SetKwData{Left}{left}\SetKwData{This}{this}\SetKwData{Up}{up}
\SetKwFunction{Union}{Union}\SetKwFunction{FindCompress}{FindCompress}
\SetKwInOut{Input}{Input}\SetKwInOut{Output}{Output}
\Input{Source dataset $D_s = \{(\bmx_i^s, \bmy_i^s)\}_{i=1}^{n_s}$ with $C$ categories, target dataset $D_t = \{(\bmx_i^t)\}_{i=1}^{n_t}$ and network $G_\theta$}
\Output{Target labels $\{\hat{\bmy}^t_i\}_{i=1}^{n_t}$}
% Apply \emph{Invert} transformation on the source and target images; $\bmx:=Inv(\bmx)$ (see Sec. 3.2)\\
Train $G_\theta$ using $D_s$ with the Gaussian Mixture loss $\cL_{gm}$ in Eq. 1.\\
\For{each epoch $t = 1, 2,...,T$}{
Using Eq. 2, generate target dataset predictions and select $\frac{t}{T}.\frac{n_t}{C}$ highest confidence predictions from every category and create pseudo label set $\tilde{Y} = \{\tilde{\bmy}_i\}_{i=1}^{\tilde{n}}$. (see Sec. Approach)\;
Apply \emph{Confidence} filter $\bar{Y} = Confidence(\tilde{Y})$ (see Sec. Approach)\; 
Apply \emph{Conformity} filter $\bar{\bar{Y}} = Conformity(\bar{Y})$ (see Sec. Approach)\;
Apply \emph{Consistency} filter $\bar{\bar{\bar{Y}}} = Consistency(\bar{\bar{Y}})$ (see Sec. Approach)\;
Calculate $\lambda$ using Eq. 6; \\
Train $G_\theta$ using loss functions $\cL_{gm}^s(\bmx^s, \bmy^s)$ and $\lambda \times\cL_{gm}^t(\bar{\bar{\bar{\bmx}}}^t, \bar{\bar{\bar{\bmy}}}^t)$\ \\
\qquad where $\cL_{gm}^s$ and $\cL_{gm}^t$ are loss functions for the source and target data respectively (see Eq. 5); \\}
Predict target labels $\hat{\bmy}^t$ using $G_\theta$\;
\Return $\{\hat{\bmy}^t_i\}_{i=1}^{n_t}$
\caption{Domain Adaptation Using Pseudo Labels}
\label{method_algorithm}
\end{algorithm}
